# Supplementary material for: Numerical simulations of acoustically generated gravitational waves at a first order phase transition
Source: arXiv:1504.03291 ancillary file (2016-01-07)

# Supplementary Material for "Numerical simulations of acoustically generated gravitational waves at a first order phase transition"

(Dated: April 14, 2015)

In this supplementary material we present power spectra for all simulations listed in Table II in the main paper. For each simulation, we give longitudinal fluid and gravitational wave power spectra for the same times as in the results section, namely $500/T_\mathrm{c}$, $1000/T_\mathrm{c}$, $1500/T_\mathrm{c}$, $2000/T_\mathrm{c}$ and $2500/T_\mathrm{c}$. In some cases only a subset of times is available. We also include time series of $\overline{U}_\phi$ and $\overline{U}_\mathrm{f}$ in each section.

While the paper is intended to be self-contained we provide this in the interests of completeness. Each series of graphs is shown on the same axis range for every parameter choice, with the exception of the 'intermediate' run at the end where additional range was required.

## I. WEAK TYPE TRANSITIONS

### A. $\eta/T_\mathbf{c} = 0.06$, $v_\mathbf{w} = 0.83$

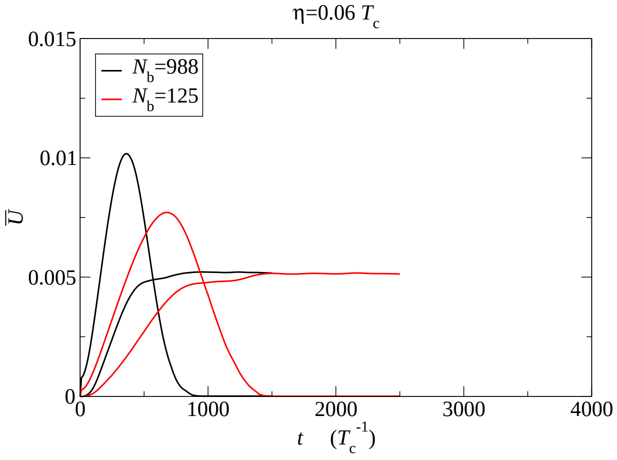


#### 1. $N_b = 988$

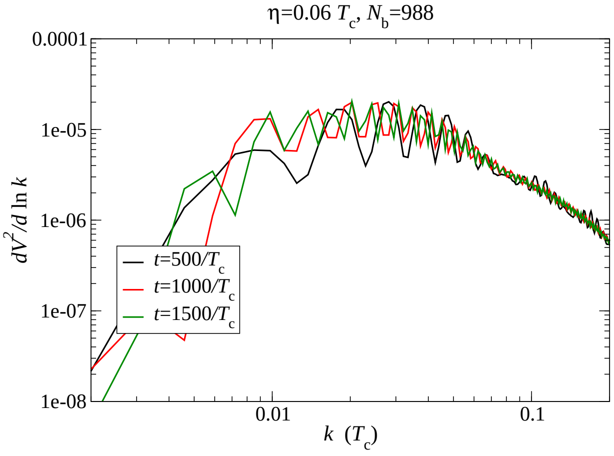


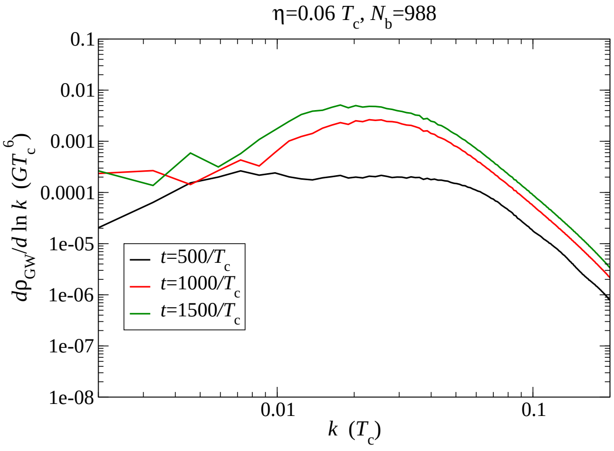

### 2. $N_b = 125$

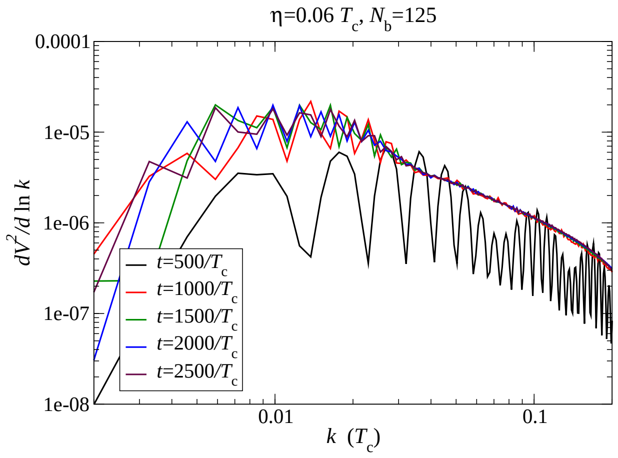


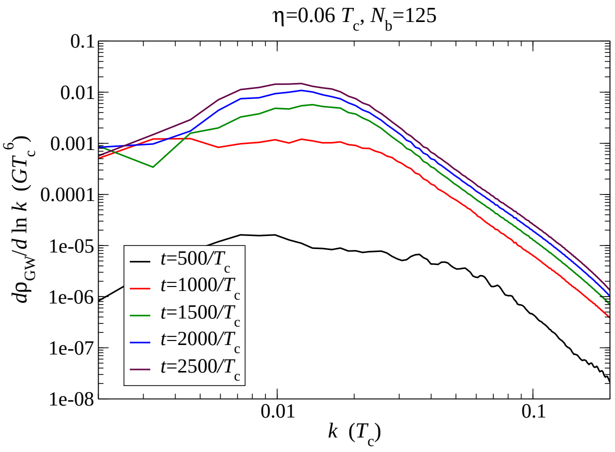


## B. $\eta/T_c = 0.1$, $v_w = 0.68$

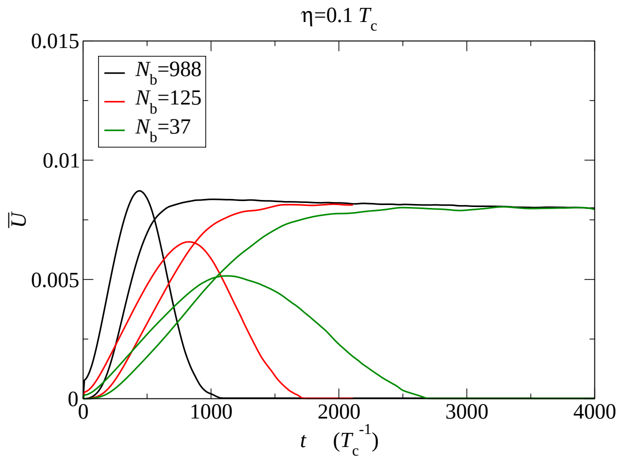


### 1. $N_b = 988$

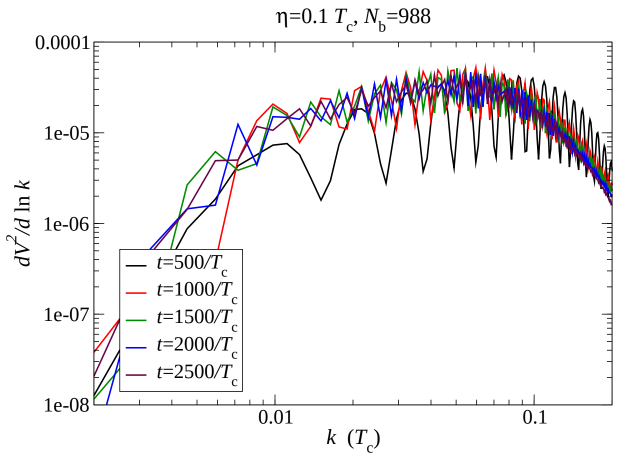


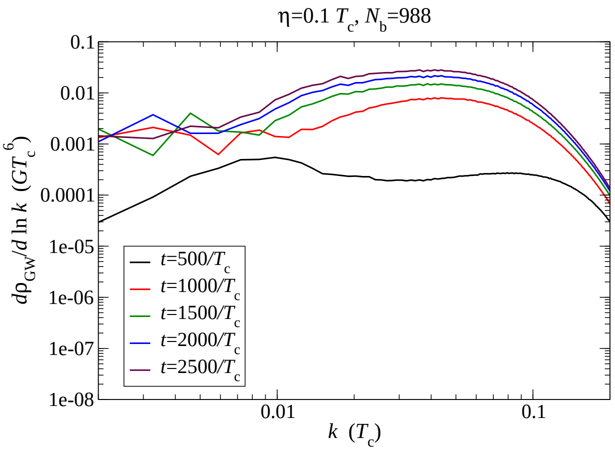

### 2. $N_b = 125$

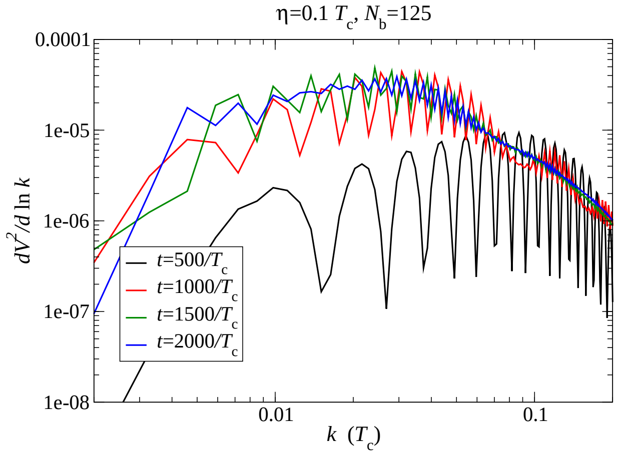


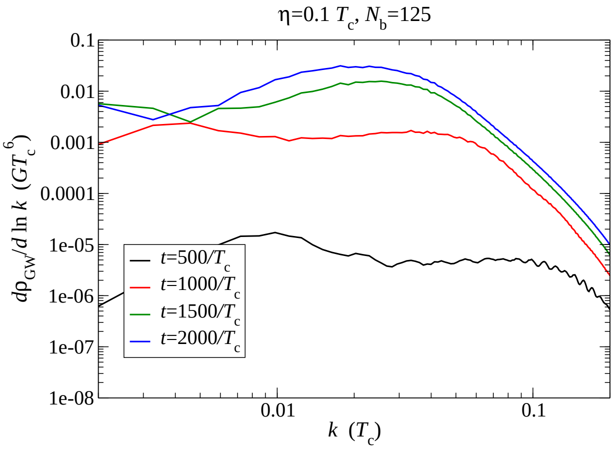


### 3. $N_b = 37$

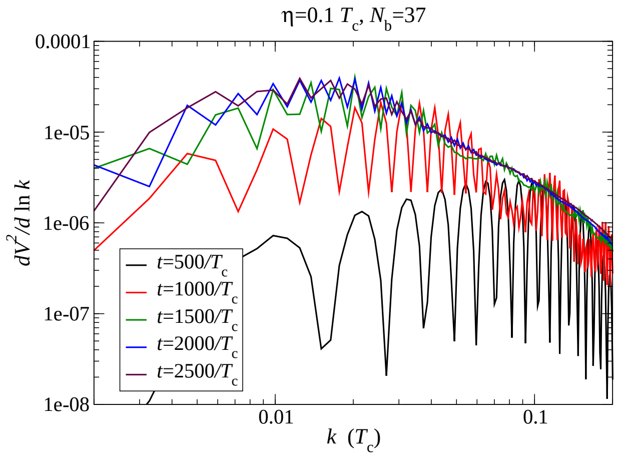


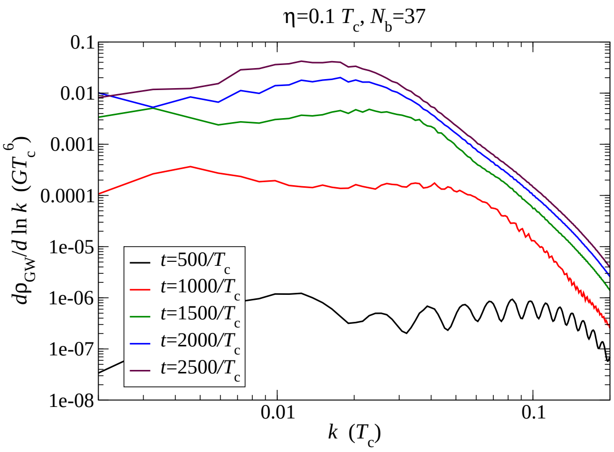


## C. $\eta/T_\mathbf{c} = 0.121$, $v_\mathbf{w} = 0.59$

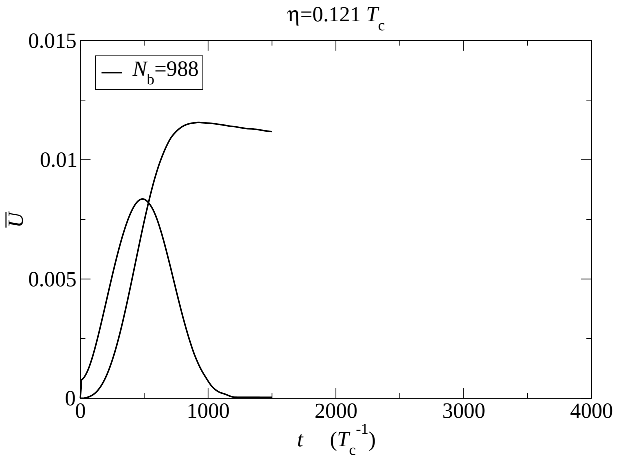

### 1. $N_b = 988$

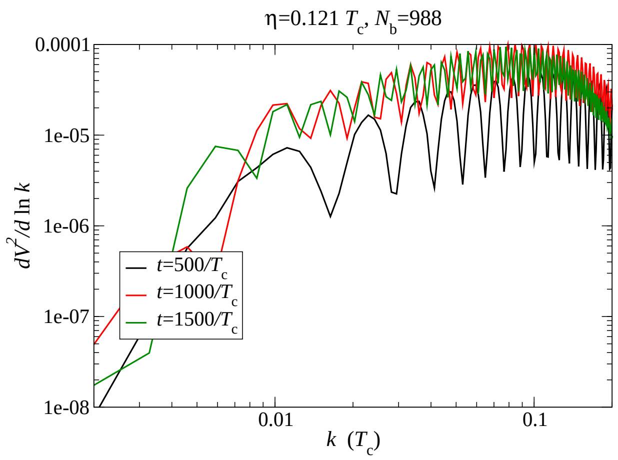


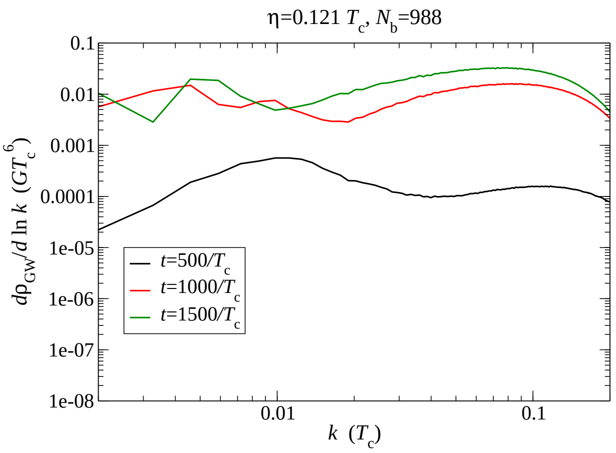


## D. $\eta/T_\mathbf{c} = 0.15$, $v_\mathbf{w} = 0.54$

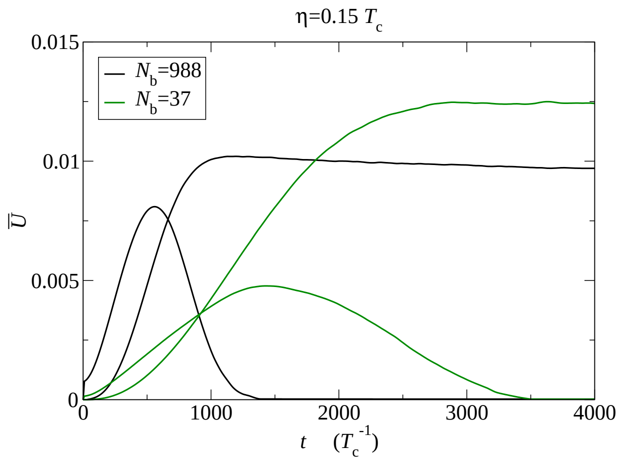


### 1. $N_b = 988$

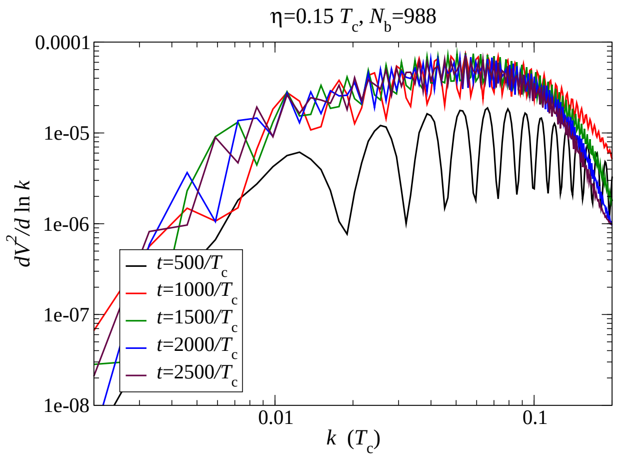


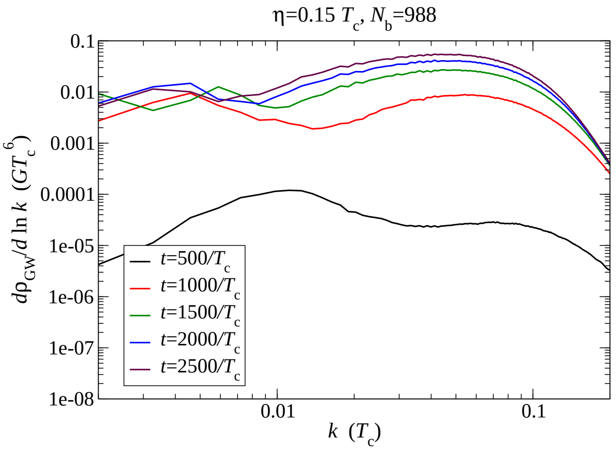

### 2. $N_b = 37$

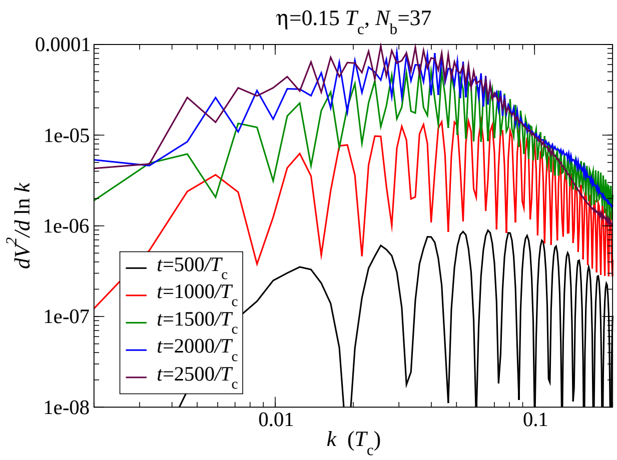


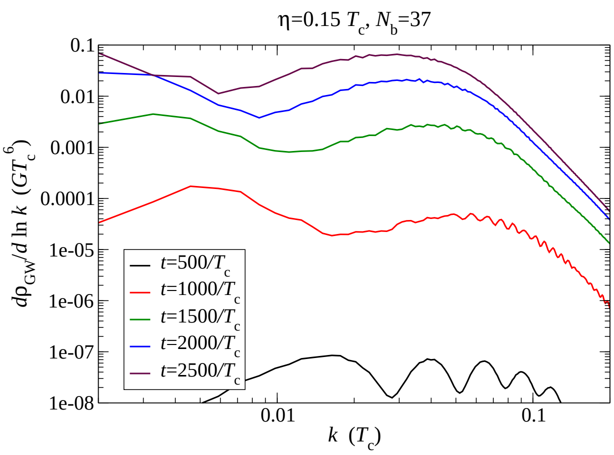


## E. $\eta/T_c = 0.2$, $v_w = 0.44$

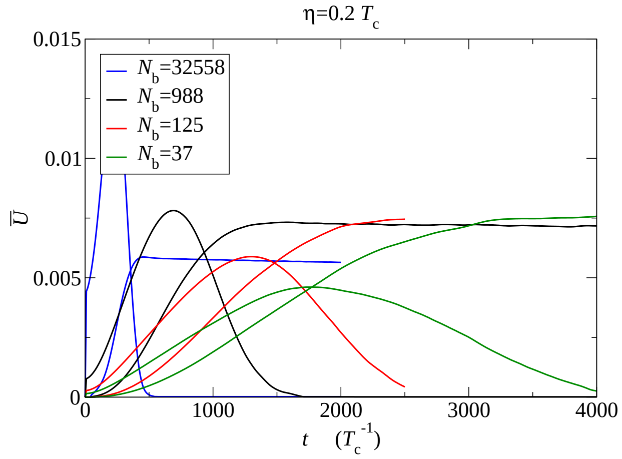


### 1. $N_b = 32558$

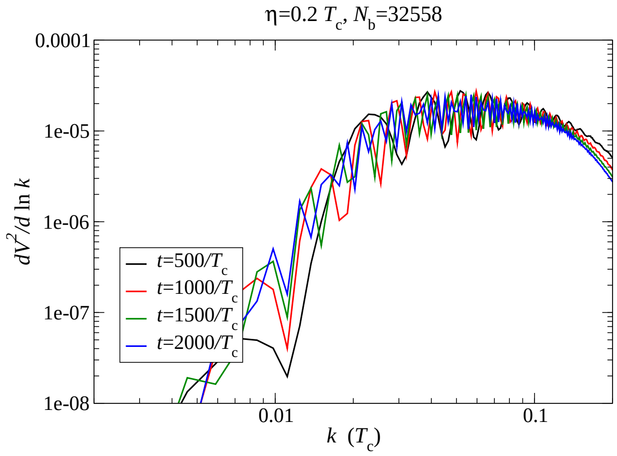


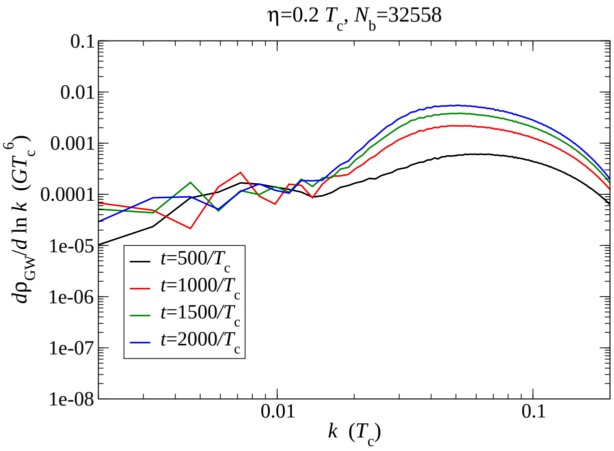

### 2. $N_b = 988$

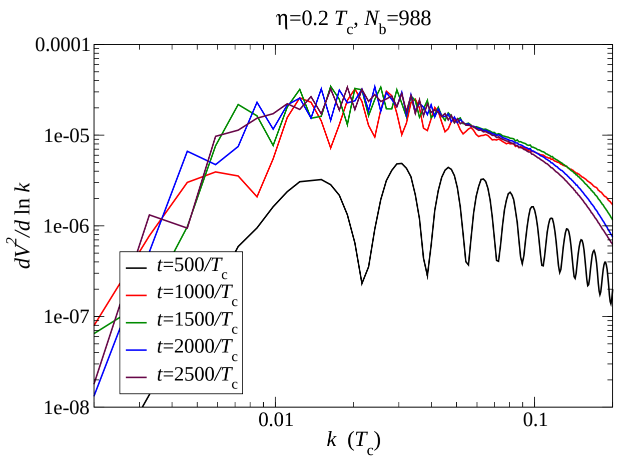


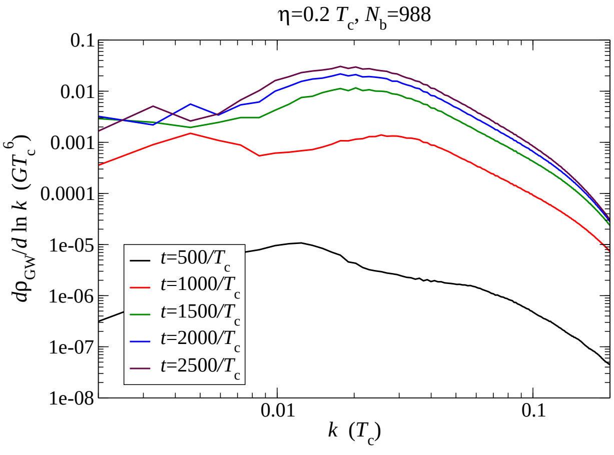


### 3. $N_b = 125$

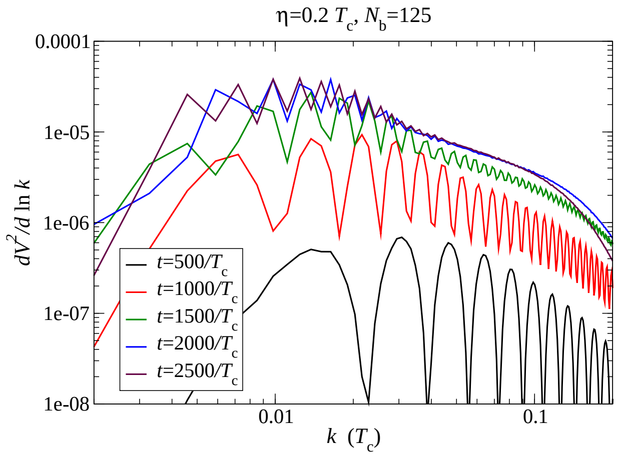


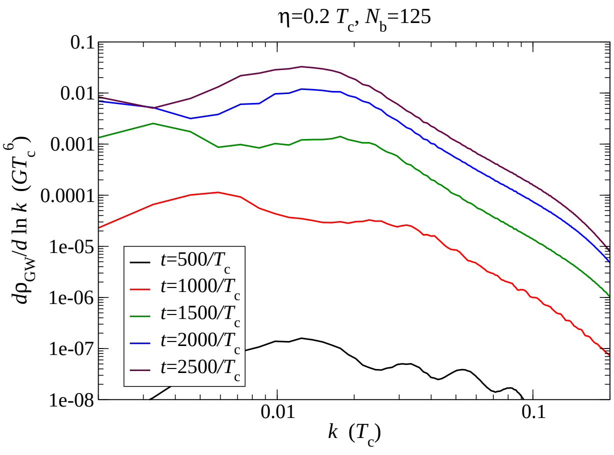


### 4. $N_b = 37$

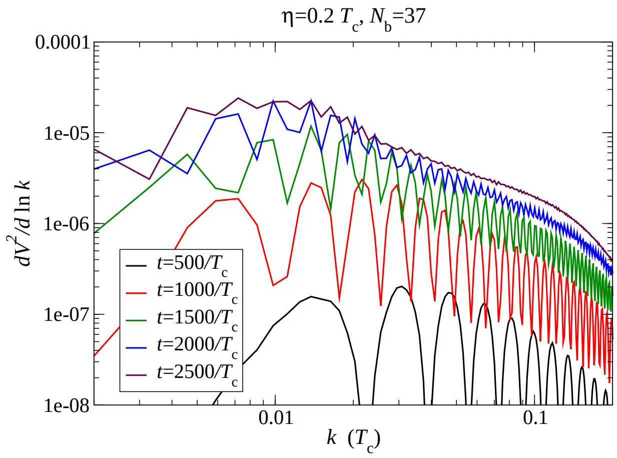


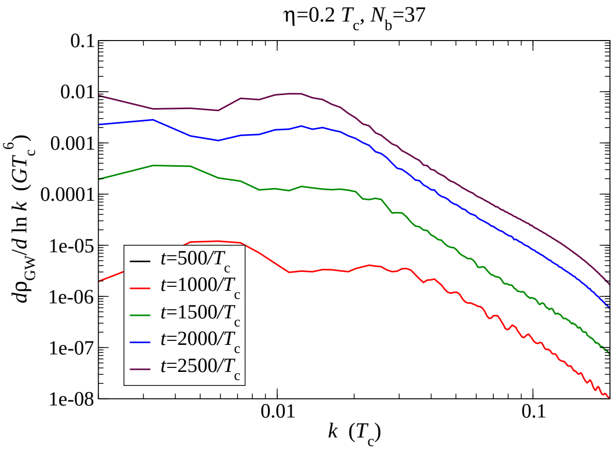

### F. $\eta/T_c = 0.4$, $v_w = 0.24$

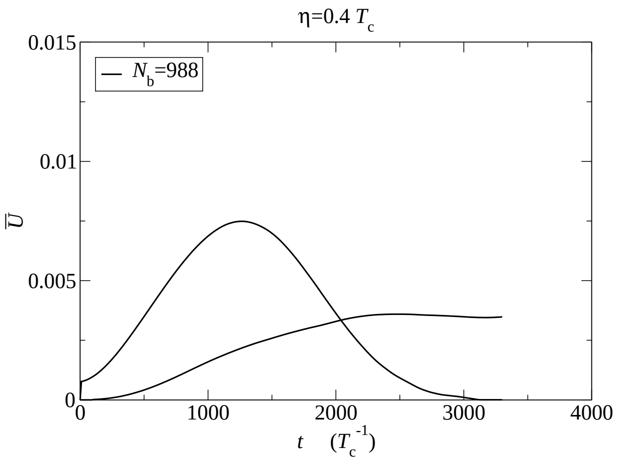


#### 1. $N_b = 988$

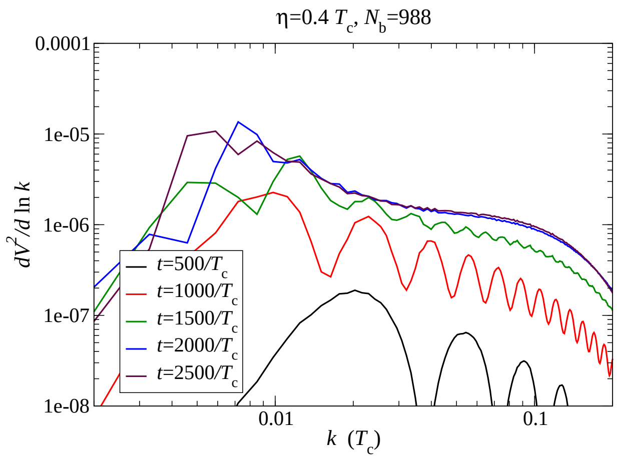


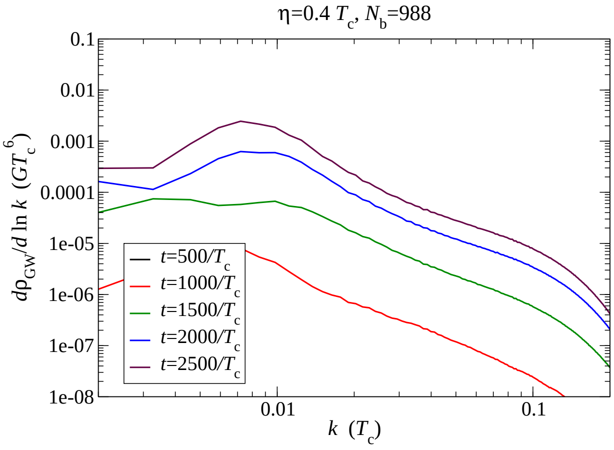


## II. WEAK (SCALED) TYPE TRANSITION

### A. $\eta/T_c = 0.4$, $v_w = 0.44$

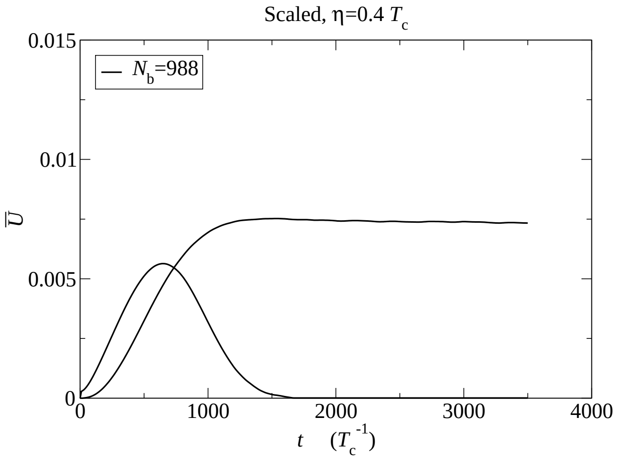

### 1. $N_b = 988$

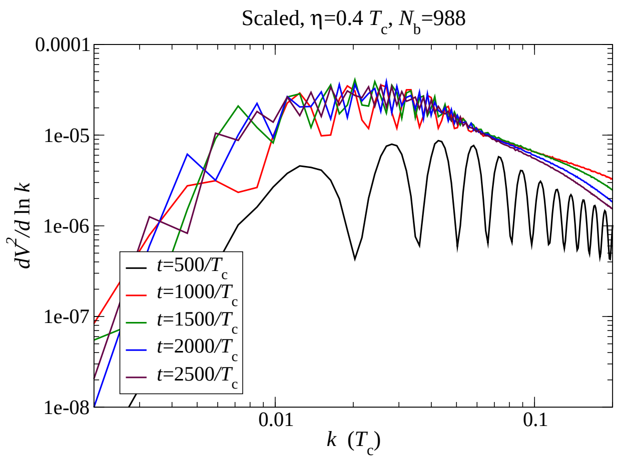


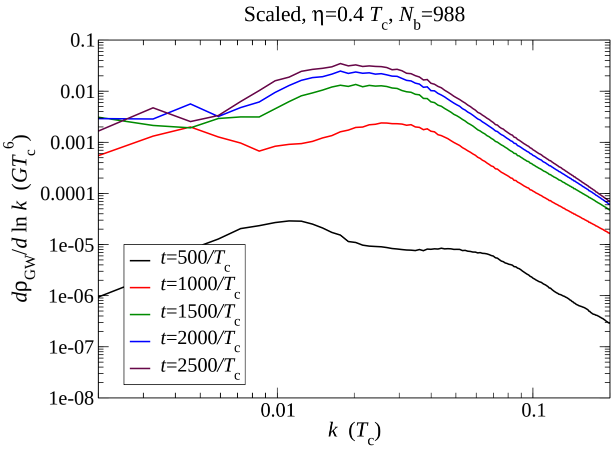


## III. INTERMEDIATE TYPE TRANSITION

### A. $\eta/T_c = 0.4$, $v_w = 0.44$

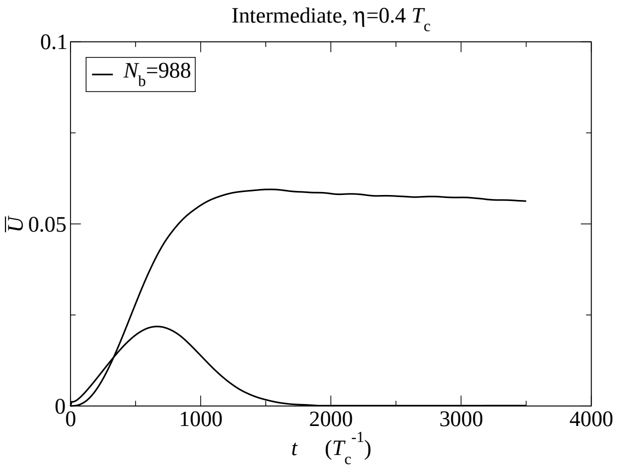


### 1. $N_b = 988$

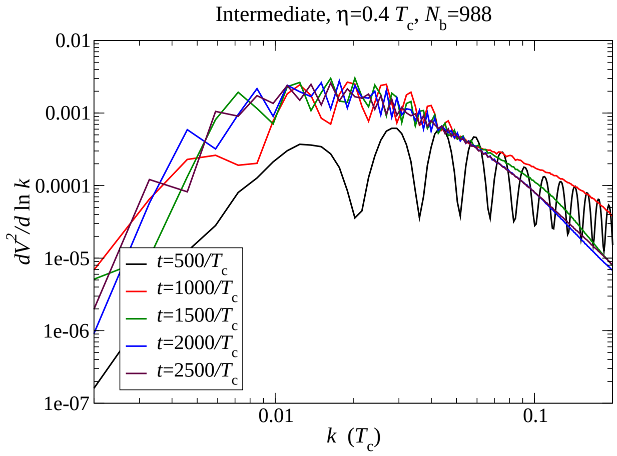


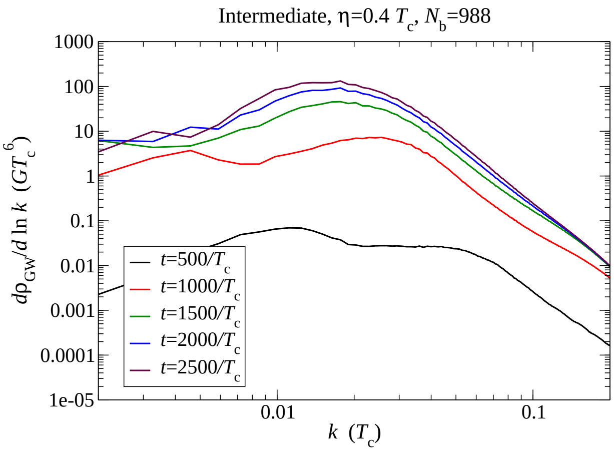

Supplement: Supplementary file 1 [file supplementary.pdf]
